# Supplementary material for: CrackSegFlow: Controllable Flow Matching Synthesis for Generalizable Crack Segmentation with a 50K Image-Mask Benchmark
Source: arXiv:2601.03637 ancillary file (2026-01-11)
Supplement: Supplementary file 1 [file CrackSegFlow__supplementary_materials_.pdf]

# Supplementary Material for:
# *CrackSegFlow: Controllable Flow Matching Synthesis for Generalizable Crack Segmentation with a 50K Image–Mask Benchmark*

Babak Asadi[a,b], Peiyang Wu[a,b], Mani Golparvar-Fard[a,b], Ramez Hajj[a]

[a] *Department of Civil and Environmental Engineering, Grainger College of Engineering, University of Illinois Urbana–Champaign, Urbana, IL, 61801, USA*
[b] *Department of Computer Science, Grainger College of Engineering, University of Illinois Urbana–Champaign, Urbana, IL, 61801, USA*

---

---

## S1. Additional in-domain qualitative results

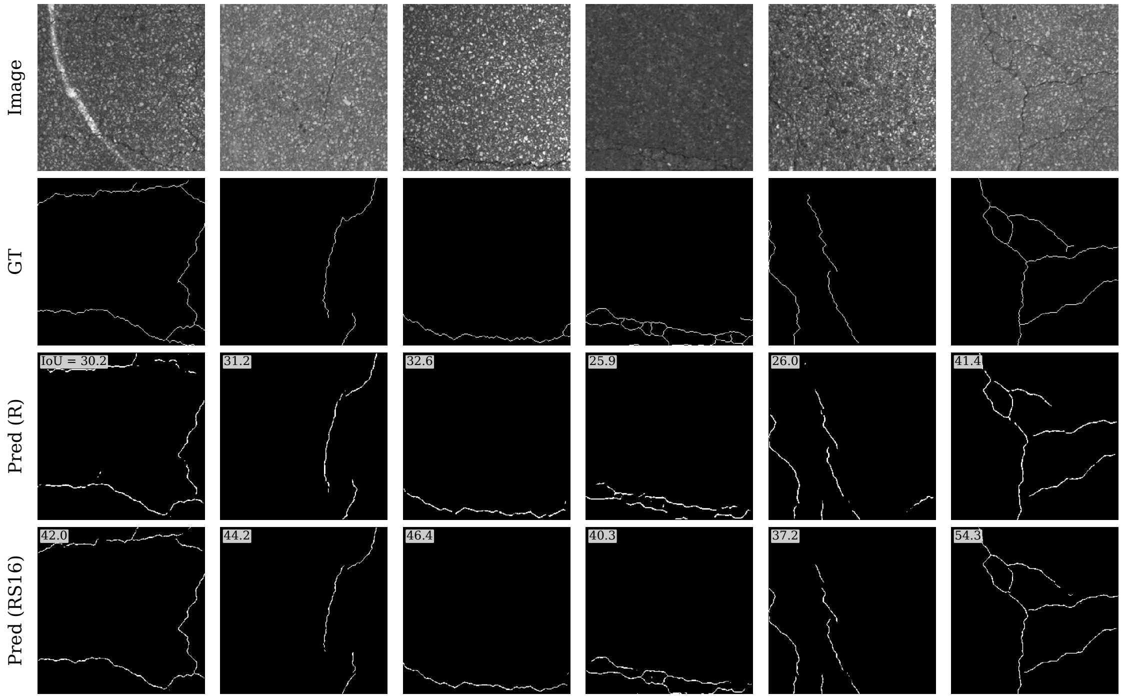


**Fig. S1:** In-domain qualitative comparison on CrackLS315. Adding synthesized pairs reduces spurious responses while preserving thin-structure continuity and 1-pixel centerline fidelity.

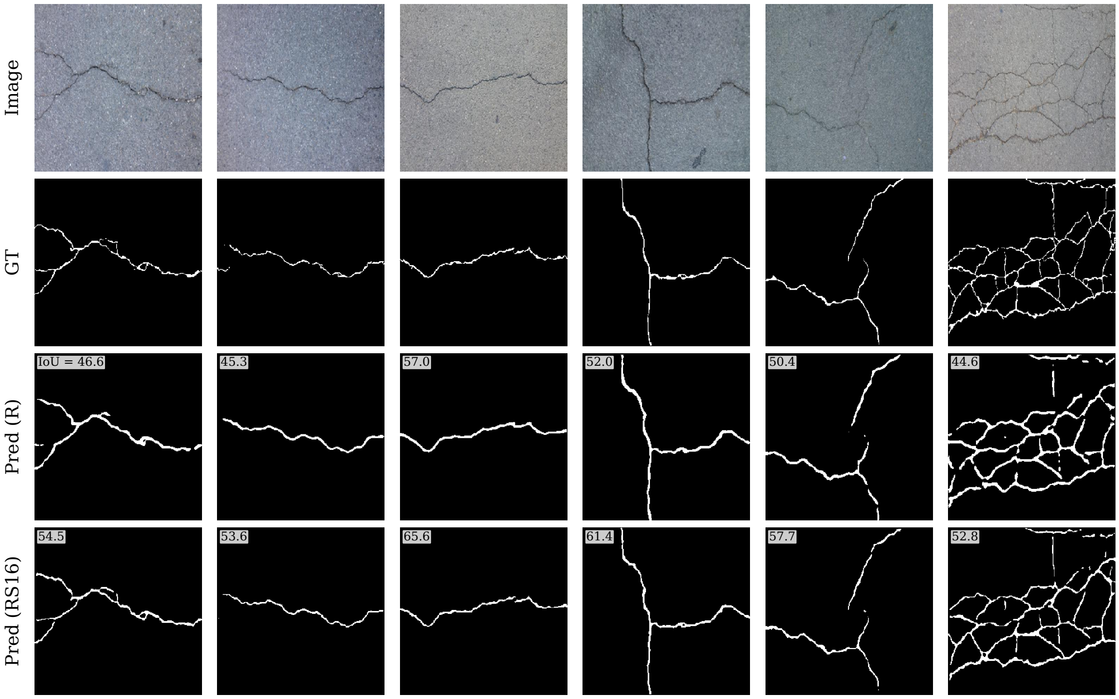


**Fig. S2:** In-domain qualitative comparison on CFD. Adding synthesized pairs suppresses texture-driven false positives and improves crack connectivity under varied surface patterns.

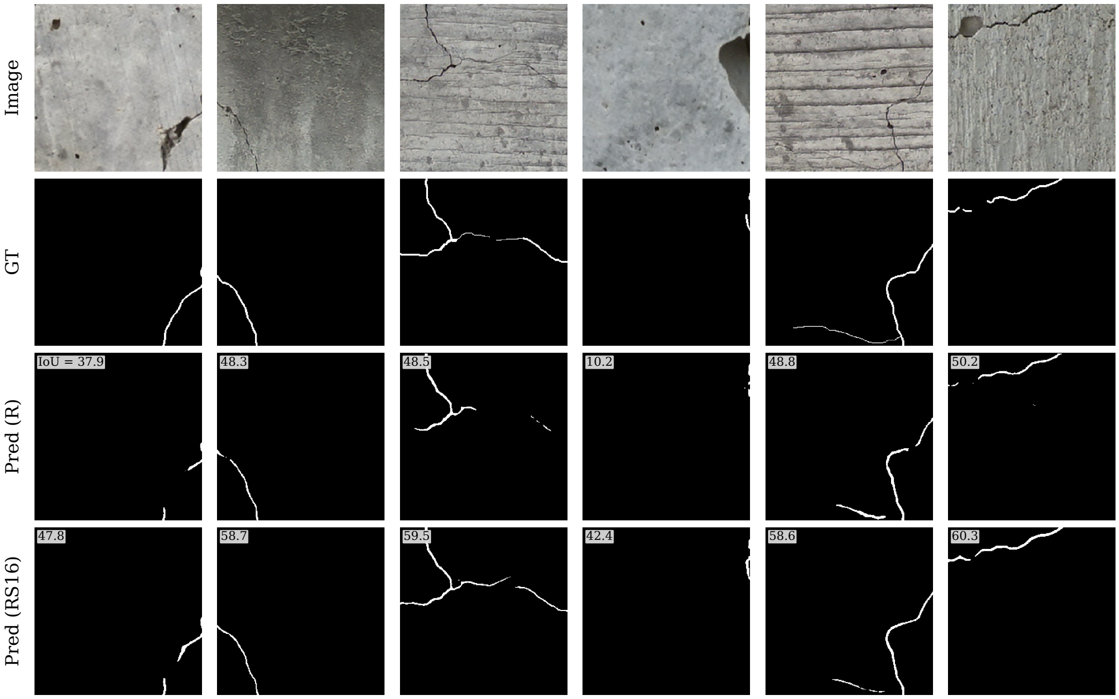


**Fig. S3:** In-domain qualitative comparison on S2DS (concrete domain). Adding synthesized pairs reduces spurious detections on concrete texture while maintaining thin-crack fidelity.

## S2. Additional cross-domain qualitative results

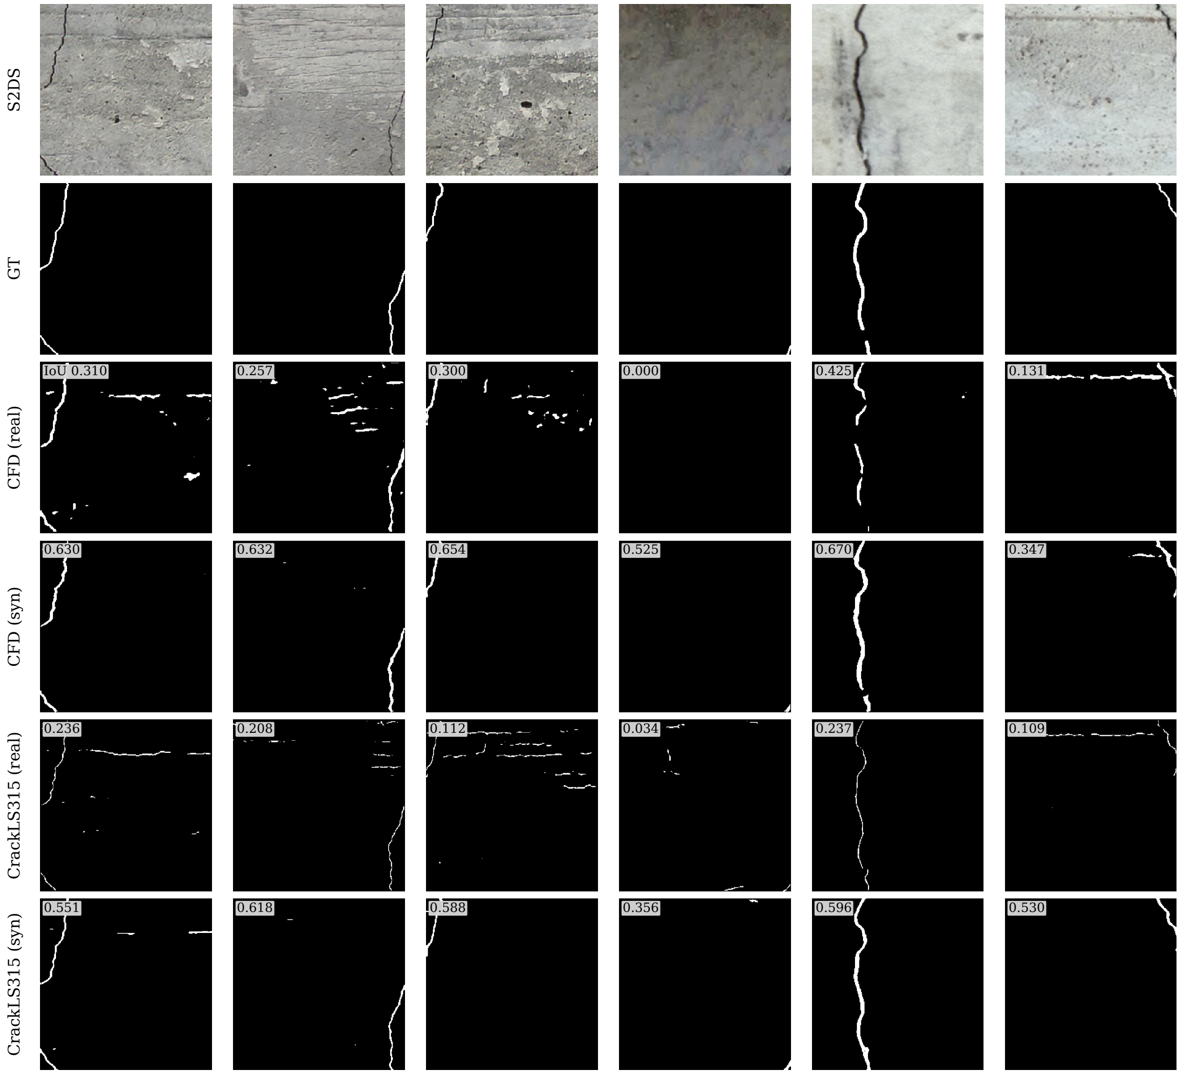


**Fig. S4:** Cross-domain qualitative results on S2DS (target) using models trained on CFD and CrackLS315 (sources). Rows show the target image, ground-truth mask (cracks in white), and predictions from real-only and target-guided syn-only training for each source. IoU overlays report per-image agreement with the ground truth.

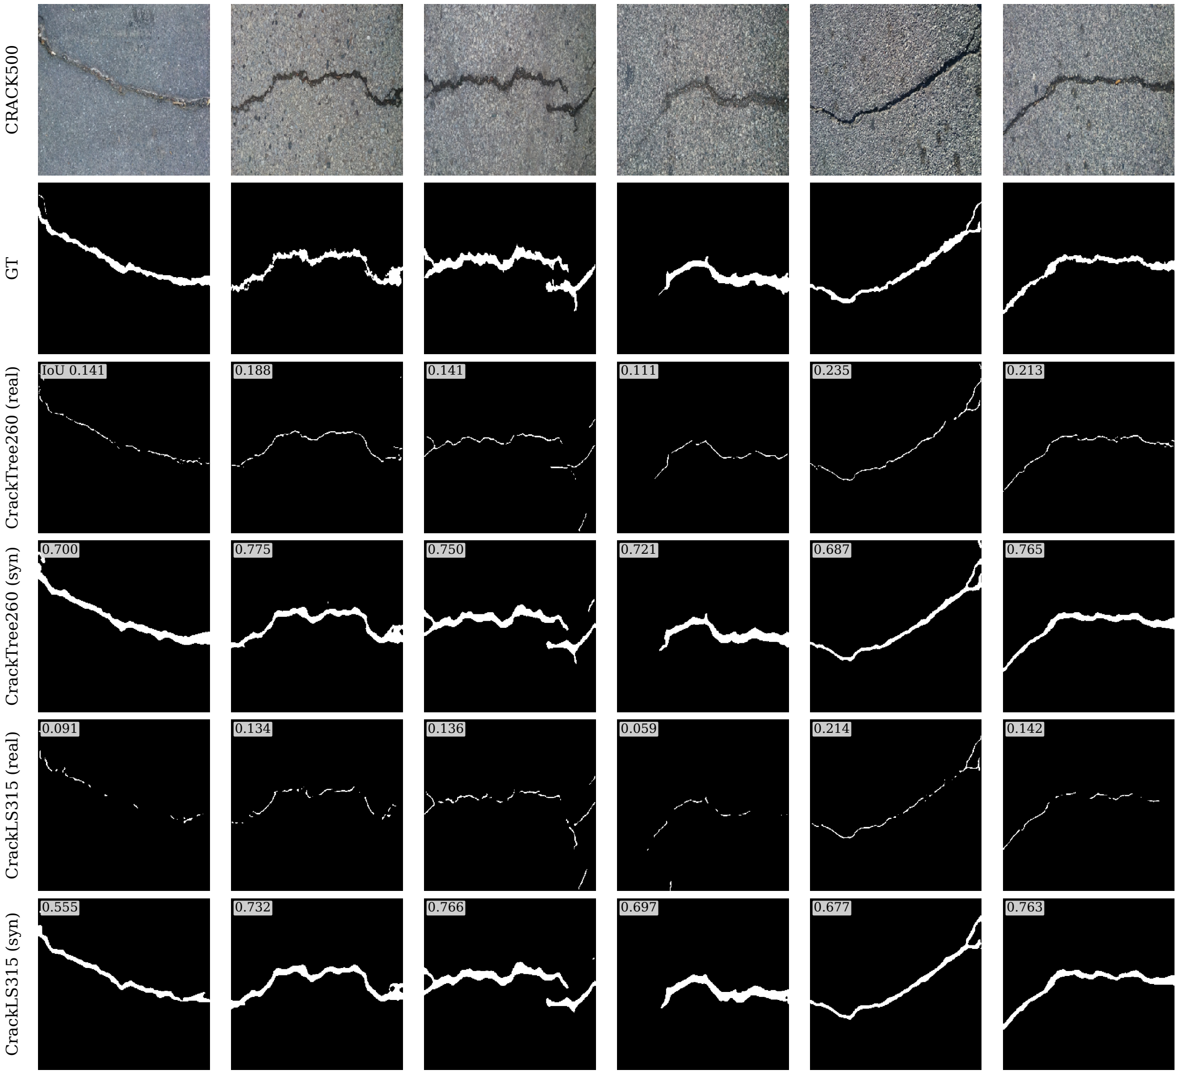


**Fig. S5:** Cross-domain qualitative results on CRACK500 (target) using models trained on CrackTree260 and CrackLS315 (sources). Rows show the target image, ground-truth mask (cracks in white), and predictions from real-only and target-guided syn-only training for each source. IoU overlays facilitate direct visual–quantitative comparison.
